# Supplementary material for: LLARVA: Vision-Action Instruction Tuning Enhances Robot Learning
Source: arXiv:2406.11815 source file (2024-06-17)
Supplement: Supplementary file 1 [file appendix.tex]

\section{More Details of Our Dataset}
